# Supplementary material for: SafeEar: Content Privacy-Preserving Audio Deepfake Detection
Source: arXiv:2409.09272 source file (2024-09-14)
Supplement: Supplementary file 1 [file 13_additional_cost.tex]

\begin{table}[t!]
\centering
\small
 
% \resizebox{0.85\linewidth}{!}{
% \begin{threeparttable}[t]
% \renewcommand{\TPTminimum}{\linewidth}
\setlength{\tabcolsep}{6pt}
\setlength{\abovecaptionskip}{0pt}% 
\setlength{\belowcaptionskip}{0pt}%
\color{blue}
\caption{\label{tab:additional_cost}Additional cost of \sys compared with baseline methods: RTF and FLOPs.}
\begin{threeparttable}
\begin{tabular}{@{}llcc@{}}
\toprule[1.2pt]
\multicolumn{1}{c}{\textbf{Type}} & \multicolumn{1}{c}{\textbf{Method}} & \multicolumn{1}{c}{\textbf{RTF} $\downarrow$} & \multicolumn{1}{c}{\textbf{FLOPs} $\downarrow$} \\
\midrule[1pt]
\multirow{2}{*}{\textbf{End-to-End}}   & AASIST  &  0.0155  &  45.49T  \\
& Rawformer   &   0.0145   &  5.24T  \\
\midrule
\multirow{2}{*}{\textbf{Pipeline}}        & Wav2vec2+Transformer   &    0.0111   &  47.05T  \\
& SafeEar (Ours)   &   0.0366  &  62.76T  \\
\bottomrule[1.2pt]
\end{tabular}
% \begin{tablenotes}[flushleft]
%     \item[] \vspace{-2pt}\hspace{-2pt}\small 
%     (1) $^\natural$: RTF is short for ``Real-Time Factor'', RTF=$T_{detect}$/$T_{audio}$, indicating how fast the model can process audio input, where $T_{audio}$ is the duration of the original audio, and $T_{detect}$ is the time to detect the authenticy of the audio.\\
%     (2) $\ddagger$: FLOPs quantify the number of floating point operations, is hardware-agnostic metric to compare the inherent computational demands of different models, the lower the FLOPs, the lower the algorithmic complexity the model has.
% \end{tablenotes}
\end{threeparttable}
\end{table}
